# Supplementary material for: Likelihood-Free Frequentist Inference: Bridging Classical Statistics and Machine Learning for Reliable Simulator-Based Inference
Source: arXiv:2107.03920 source file (2024-11-26)
Supplement: Supplementary file 1 [file supplementary.tex]

\setcounter{page}{1}
\begin{supplement}
    \addEJS{Below we include additional results and discussions that integrate the main text of the paper ``\textit{Likelihood-Free Frequentist Inference: Bridging Classical Statistics and Machine Learning for Reliable Simulator-Based Inference}''.}
\end{supplement}

\section{Breakdown of Sources of Error in LF2I Confidence Sets}\label{sec:sources_errors}

In traditional statistical inference, confidence sets depend on the choice of  test statistic, the assumed distribution of the test statistic under the null, and the amount of available data. In LFI, however, there can be additional sources of errors. For the LF2I framework in general, \addEJS{and more specifically for \ACORE and \texttt{BFF}}, we categorize these errors as follows:
\begin{enumerate}
    \item[$e_1$:] Estimation error in learning the odds (Section~\ref{sec:learn_odds});
    \item[$e_2$:] Numerical error in evaluating the test statistic by maximization in \ACORE (Equation~\ref{eq:ACORE_statistic}) or by integration in \BFF (Equation~\ref{eq:BFF_statistic}); 
    \item[$e_3$:] Estimation error in learning the critical values (Section~\ref{sec:critical-value}) or the p-values (Section~\ref{sec:pval}).
\end{enumerate}
\paragraph{Validity and power}  \textit{Validity} is directly determined by $e_3$. As shown in Section~\ref{sec:theory}, one can construct valid confidence sets regardless of how well the test statistic is estimated, as long as the quantile regressor (Algorithm~\ref{alg:estimate_cutoffs}) or probabilistic classifier for estimating p-values  (Algorithm~\ref{alg:estimate_pvalues}) are consistent and the number of simulations $B'$ is large enough. \addEJS{In practice, we observe that the number of simulations $B^\prime$ needed to achieve correct coverage is usually much lower relative to $B$, the number of simulations needed to estimate the test statistic.} The {\em power or expected size} of the confidence set is, on the other hand, determined by both $e_1$ and $e_2$.  The error $e_1$ depends on the capacity of the classifier for estimating odds and the training sample size  $B$. The error $e_2$ is a purely numerical error and can be reduced by \addEJS{employing modern numerical optimization and integration algorithms suitable for the problem at hand. Figure~\ref{fig:gaussian_LFI_power_acrossd} -- and Supplementary Material~\ref{sec:multivariate_gaussian} in general -- offers an empirical analysis of $e_2$ on Gaussian data of increasing dimensionality.} Note that for this example we are not employing any particular numerical optimization or importance-weighted integration technique. We are simply generating a uniform grid over the parameter space and then computing the maximum or sum of relevant quantities over the grid points to evaluate the \ACORE or \BFF statistics, respectively. \addEJS{Examples in Section~\ref{sec:hep_example}, instead, used modern algorithms available from \texttt{SciPy} \cite{2020SciPy-NMeth}.}

\paragraph{Practical strategy for model selection} To mitigate all sources of errors \addEJS{for LF2I with the \ACORE and \BFF test statistics}, we proceed as follows:
\begin{enumerate}
    \item
    To estimate the odds function, select a probabilistic classifier and the number of simulations $B$ 
    based on the cross-entropy loss on held-out data;\footnote{ One can alternatively use  the integrated odds loss (Equation~\ref{eq::odds_loss}). However, as shown in Supplementary Material~\ref{app:sim_derivs}, the odds loss is much more sensitive than the cross-entropy loss to the value of the estimated odds, which can lead to the odds loss wildly fluctuating for different values of $B$.}
    \item To compute the test statistic, choose \addEJS{modern numerical optimization and integration routines, especially to avoid local minima/maxima in the computation of \texttt{ACORE};}
    \item To ensure valid confidence sets, select the quantile regressor and the train sample size $B'$ so that we achieve nominal coverage across the entire parameter space according to LF2I diagnostics (Section~\ref{sec:diagnostics}) \addEJS{on a separate set $\T^{\prime\prime}$}. 
\end{enumerate}

\section{Examples for Assumption 7}\label{app:examples_ass7}
Below, we provide some examples where Assumption \ref{assump:modelclass} holds, using well-established results for the convergence rates of commonly used regression estimators:
\begin{itemize}
    \item \cite{Kpotufe2011KNN} shows that kNN estimators are adaptive to the intrinsic dimension $d$ under certain conditions. When $\hat \P$ is a kNN estimator with $\P$ in a class of Lipschitz continuous functions, Assumption \ref{assump:modelclass} holds with $\kappa=2$. More generally, with $\P$ in a H{\H o}lder space with parameter $0 < \beta \leq 1.5$, Assumption \ref{assump:modelclass} holds with $\kappa=2\beta$  (\cite{Gyorfi2006rates,Ayano2012rates}).
    \item \cite{KpotufeGarg2013kernelreg} show that under certain conditions, when  $\hat \P$  is a kernel regression estimator with $\P$ in a class of Lipschitz continuous functions, Assumption \ref{assump:modelclass} holds with $\kappa=2$ and $d$ the intrinsic dimension of the data. More generally, with $\P$ in a H{\H o}lder space with parameter $0 < \beta \leq 1.5$, Assumption \ref{assump:modelclass} holds with $\kappa=2\beta$  \cite{Gyorfi2006rates}.
    \item When $\hat \P$ is a local polynomial regression estimator with $\P$ in a Sobolev space with smoothness $\beta$, Assumption \ref{assump:modelclass} holds with $\kappa=\beta$, where $d$ is the manifold dimension  \cite{BickelLi2007rates}.
    \item \cite{Biau2012rates} shows that under certain conditions, when $\hat \P$ is a random forest estimator with $D$ covariates with $\P$ in a class of Lipschitz continuous functions, Assumption \ref{assump:modelclass} holds with $\kappa=2$ when the number of relevant features $d \leq D/2$.
\end{itemize}
More examples can be found in \cite{Gyorfi2006rates}, \cite{Tsybakov2009rates} and \cite{Devroye2013rates}.

\section{Gaussian Mixture Model Example}\label{app:gmm_app}

\begin{figure}[t!]
    \centering
    \hspace*{-1.4cm}    
    \includegraphics[width=1.2\textwidth]{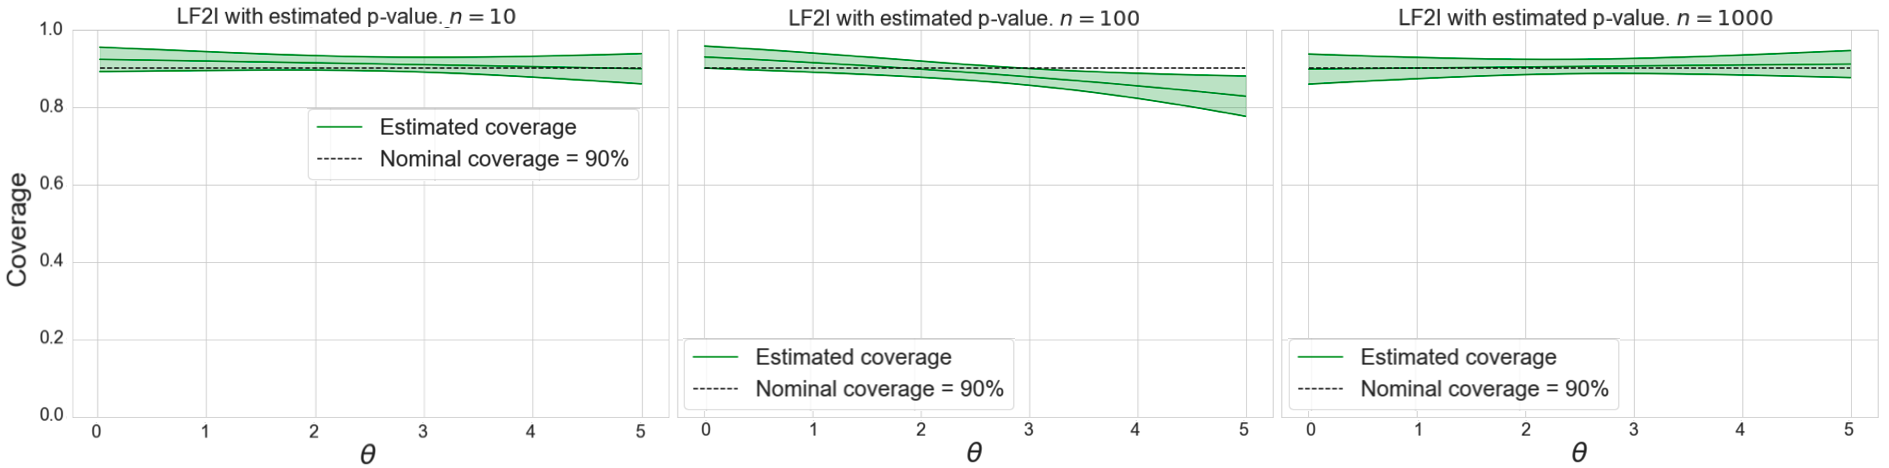}
    \caption{GMM example with sample size $n=10$ (\textit{left}), $n=100$ (\textit{center}) and $n=1000$ (\textit{right}) and confidence sets constructed using p-value estimation. The plots show the estimated coverage across $\Theta$ of 90\% confidence sets for $\theta$. As before, conditional coverage is estimated using the diagnostic branch of the LF2I framework.}
    \label{fig:gmm_pvalues}
\end{figure}

Here we (i) provide details on the algorithms used to estimate critical values and coverage in Figures~\ref{fig:GMM_coverage} and~\ref{fig:critical_61}, (ii) discuss results of experiments which account for asymmetric mixtures, and (iii) include results for applying p-value estimation to the problem in Section~\ref{sec:GMM}. \\
\\
Regarding (i): The quantile regressor used to estimate $C_{\theta_0}$ is a neural network, with two hidden layers and $32\times32$ neurons, which minimizes the quantile loss. Our experiments showed that using quantile boosted regression trees led to equivalent results, but we opted for NNs due to their inherent smoothing capabilities, which resulted in stabler estimates of the conditional quantile function. The algorithm used to estimate coverage is a binomial Generalized Additive Model (GAM) with logit link and a smoothing spline applied to the independent variable, which is $\theta$ in that setting (see Algorithm~\ref{alg:estimate_coverage}). The two-standard-deviation ($\pm 2\sigma$) prediction intervals are based on the Bayesian posterior variance of the parameters in the fitted GAM object. See documentation of the R package \texttt{MGCV} for more details. Figure~\ref{fig:critical_61} shows the estimated conditional quantile function, both via Monte-Carlo (MC) and via quantile regression. The plot also includes the upper $\alpha$ quantile of a $\chi^2_1$ distribution. Here $B^\prime$ and the number of MC simulations are both 5000\footnote{Increased with respect to the value used in Section~\ref{sec:GMM} just to make the MC and Quantile Regression curves smoother for visualization purposes. Coverage was achieved even at the previous $B^\prime=1000$.}, but the latter is again repeated for every $\theta_0$ on a fine grid. The size of each simulated sample is $n=1000$.\\
\\
Regarding (iii): So far the experiments have focused on symmetric mixtures, where both components have the same probability of being selected. We also repeated the above experiments with a mixing parameter equal to $0.8$, i.e. when the mixture is strongly unbalanced towards one mixture component but is still bi-modal. In terms of coverage, the results were qualitatively the same as those obtained in the case of symmetric mixtures.\\
\\
Regarding (iv): we conclude by showing that p-value estimation leads to confidence sets with correct conditional coverage, hence providing an alternative to critical value estimation via quantile regression. Figure~\ref{fig:gmm_pvalues} presents the results obtained on the symmetric Gaussian mixture model with samples of size $n=10, 100, 1000$, which can be compared with the right panel in Figure~\ref{fig:GMM_coverage}. Although all examples achieve correct conditional coverage, it must be noted that p-values were estimated using $B^{\prime}=10000$ to train gradient boosted classification trees, instead of $B^{\prime}=1000$ used in Section~\ref{sec:GMM} and above. In practice we have indeed observed that estimating p-values via Algorithm~\ref{alg:estimate_pvalues} requires more simulations than estimating critical values via Algorithm~\ref{alg:estimate_cutoffs}. Moreover, 
as already noted in Section~\ref{sec:pval}, the procedure for p-value estimation has to be repeated for each observed sample $D$, while critical value estimation is amortized: once the quantile regressor is fitted, it can be used for any number of observed samples.

\section{Multivariate Gaussian: Scaling with Dimension }\label{sec:multivariate_gaussian}

\begin{figure}[t!]
    \hspace*{-.3cm}
    \centering
    \includegraphics[width=1\textwidth, valign=t]{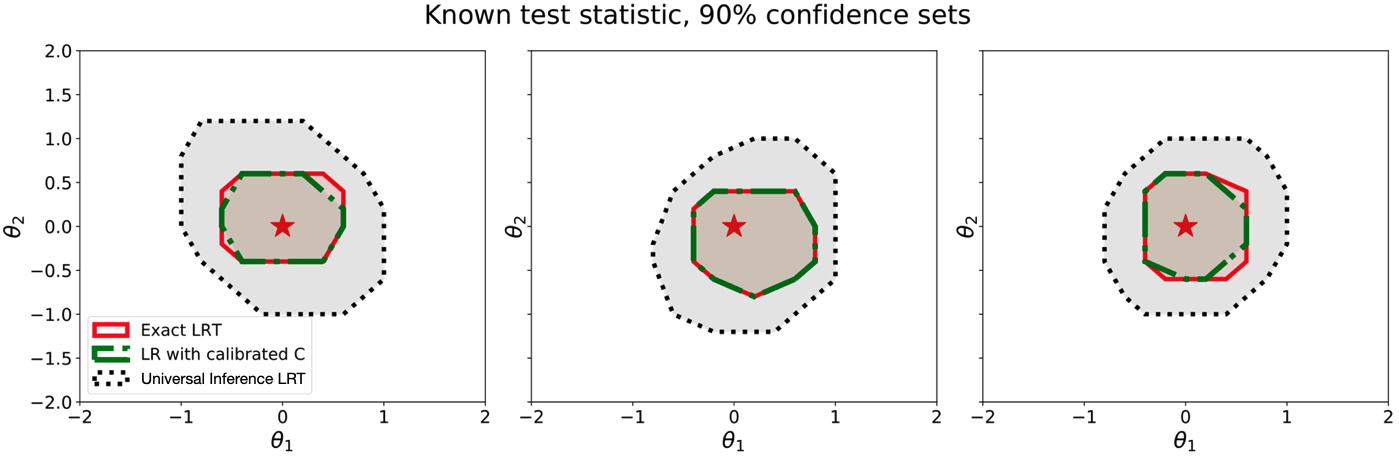}
    \caption{\small Confidence sets for known test statistics and bivariate Gaussian data. When $d=2$, our method for estimating critical values  with $B'=500$ simulations (``LR with calibrated C''; green contour) returns 90\% confidence sets that are close to the exact LRT confidence sets (red contour) and smaller than the more conservative universal inference via crossfit LRT sets (gray shading). The figures correspond to three random realizations of observed data with $n=10$ drawn from the Gaussian model with true parameter $\theta = (0,0)$ (indicated with a red star).}
    \label{fig:known_CIs}
\end{figure}

\begin{figure}[t!]
	\centering
    \textbf{Finite-sample confidence sets for known test statistic} \par\medskip
    \vspace*{-1mm}
    \resizebox{1.0\textwidth}{!}{%
	\begin{tabular}{|c|c|c|c|c|}
		\hline
		& \textbf{d=10} & \textbf{d=20} & \textbf{d=50} & \textbf{d=100} \\
		\hline
		\textbf{Coverage of LR with calibrated C} & 0.91 $\pm$ 0.03 & 0.91 $\pm$ 0.03 & 0.88 $\pm$ 0.03 & 0.88 $\pm$ 0.03 \\
		\hline
		\textbf{Coverage of Universal Inference LRT} & 0.993 $\pm$ 0.008 & 0.997 $\pm$ 0.005 & 1.000 $\pm$ 0.000 & 1.000 $\pm$ 0.000 \\
		\hline
	\end{tabular}
	}
    \includegraphics[width=0.45\textwidth]{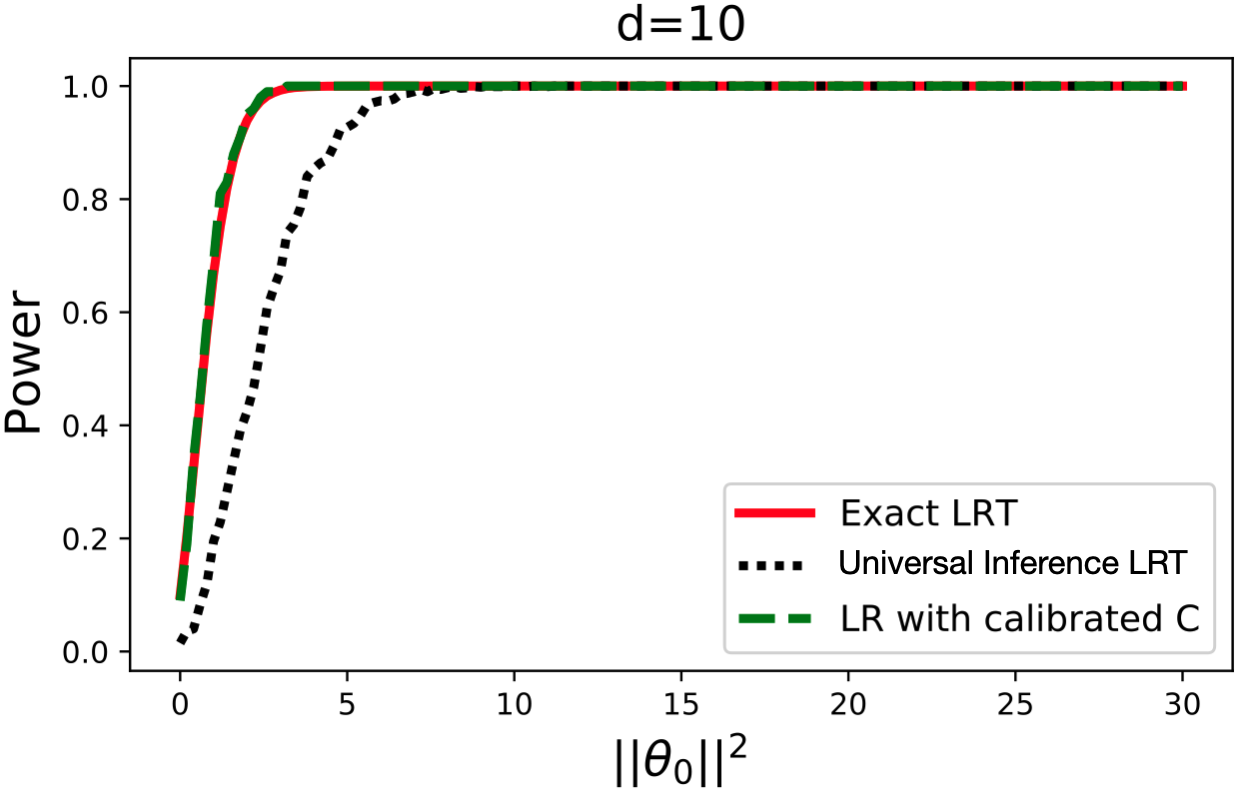}
    \includegraphics[width=0.45\textwidth]{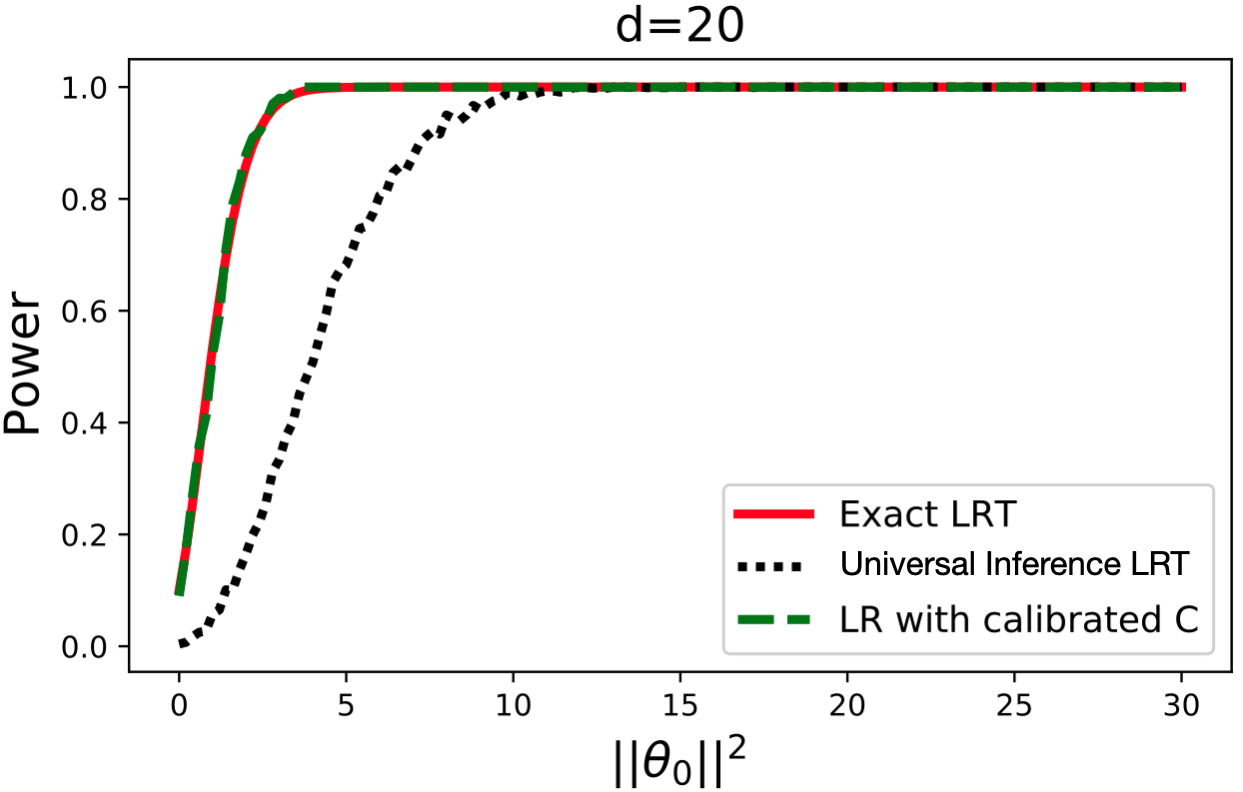}
    \includegraphics[width=0.45\textwidth]{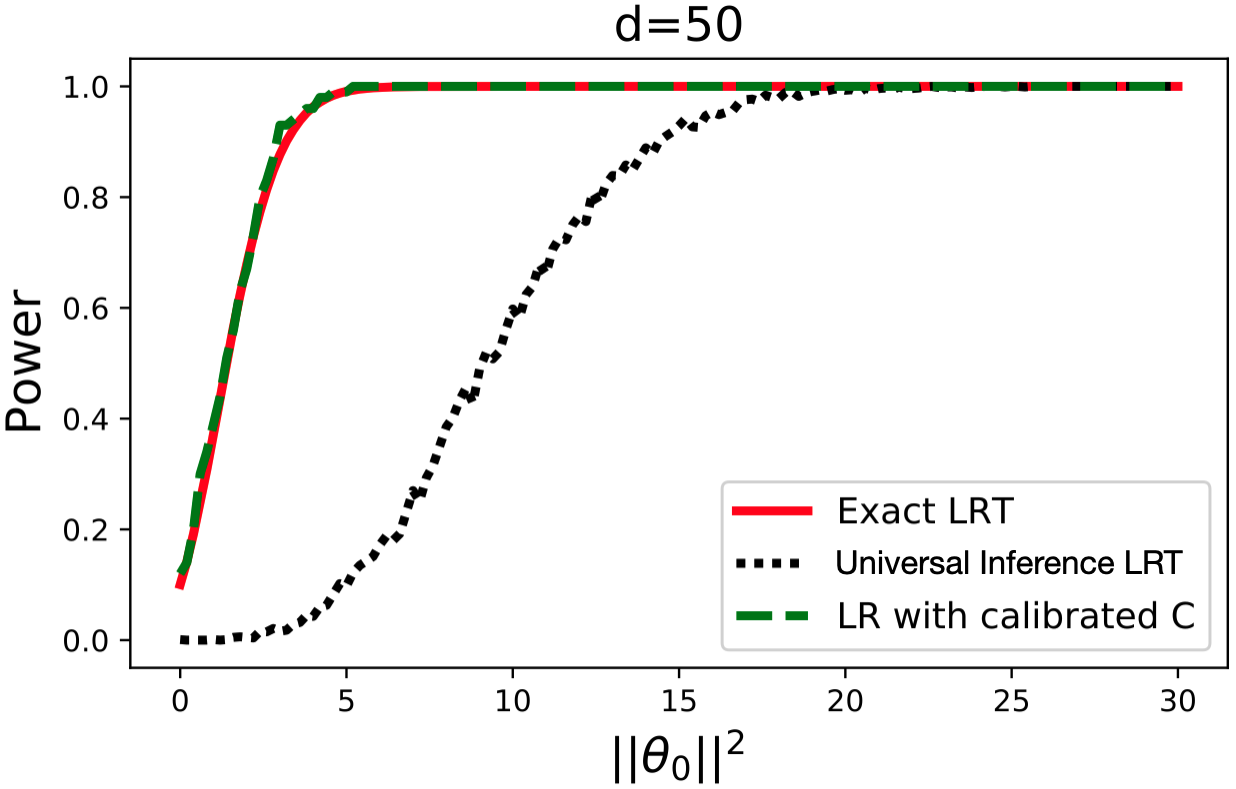}
    \includegraphics[width=0.45\textwidth]{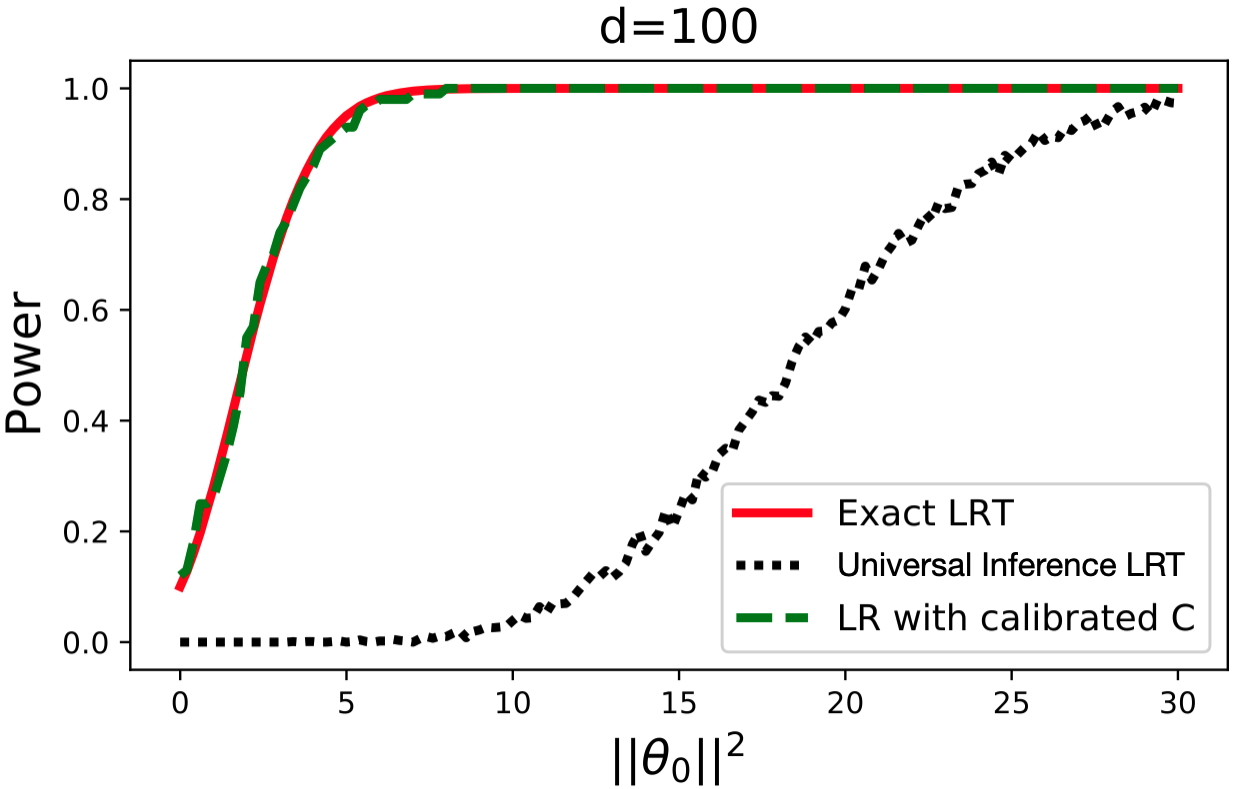}
    \caption{\small
    Confidence sets for known test statistic and $d$-dimensional Gaussian data. Coverage and power of finite-sample confidence sets constructed via exact LRT, LR with calibrated C, and universal inference via crossfit LRT (see text for details). All methods achieve the nominal coverage of $0.9$.
   When the likelihood ratio statistic is known, our construction with $B'=5000$ simulations yields the same power as the exact LRT, even in high dimensions. By calibrating the critical values, one can achieve more precise confidence sets and higher power than universal inference. See Figure~\ref{fig:known_CIs} for example confidence sets in dimension $d=2$. The difference in precision and power between the two methods increase with dimension $d$.}
	\label{fig:MVN_knownlik}
\end{figure}

\begin{figure}[t!]
	\hspace*{-.3cm}
	\centering
	\includegraphics[width=1\textwidth, valign=t]{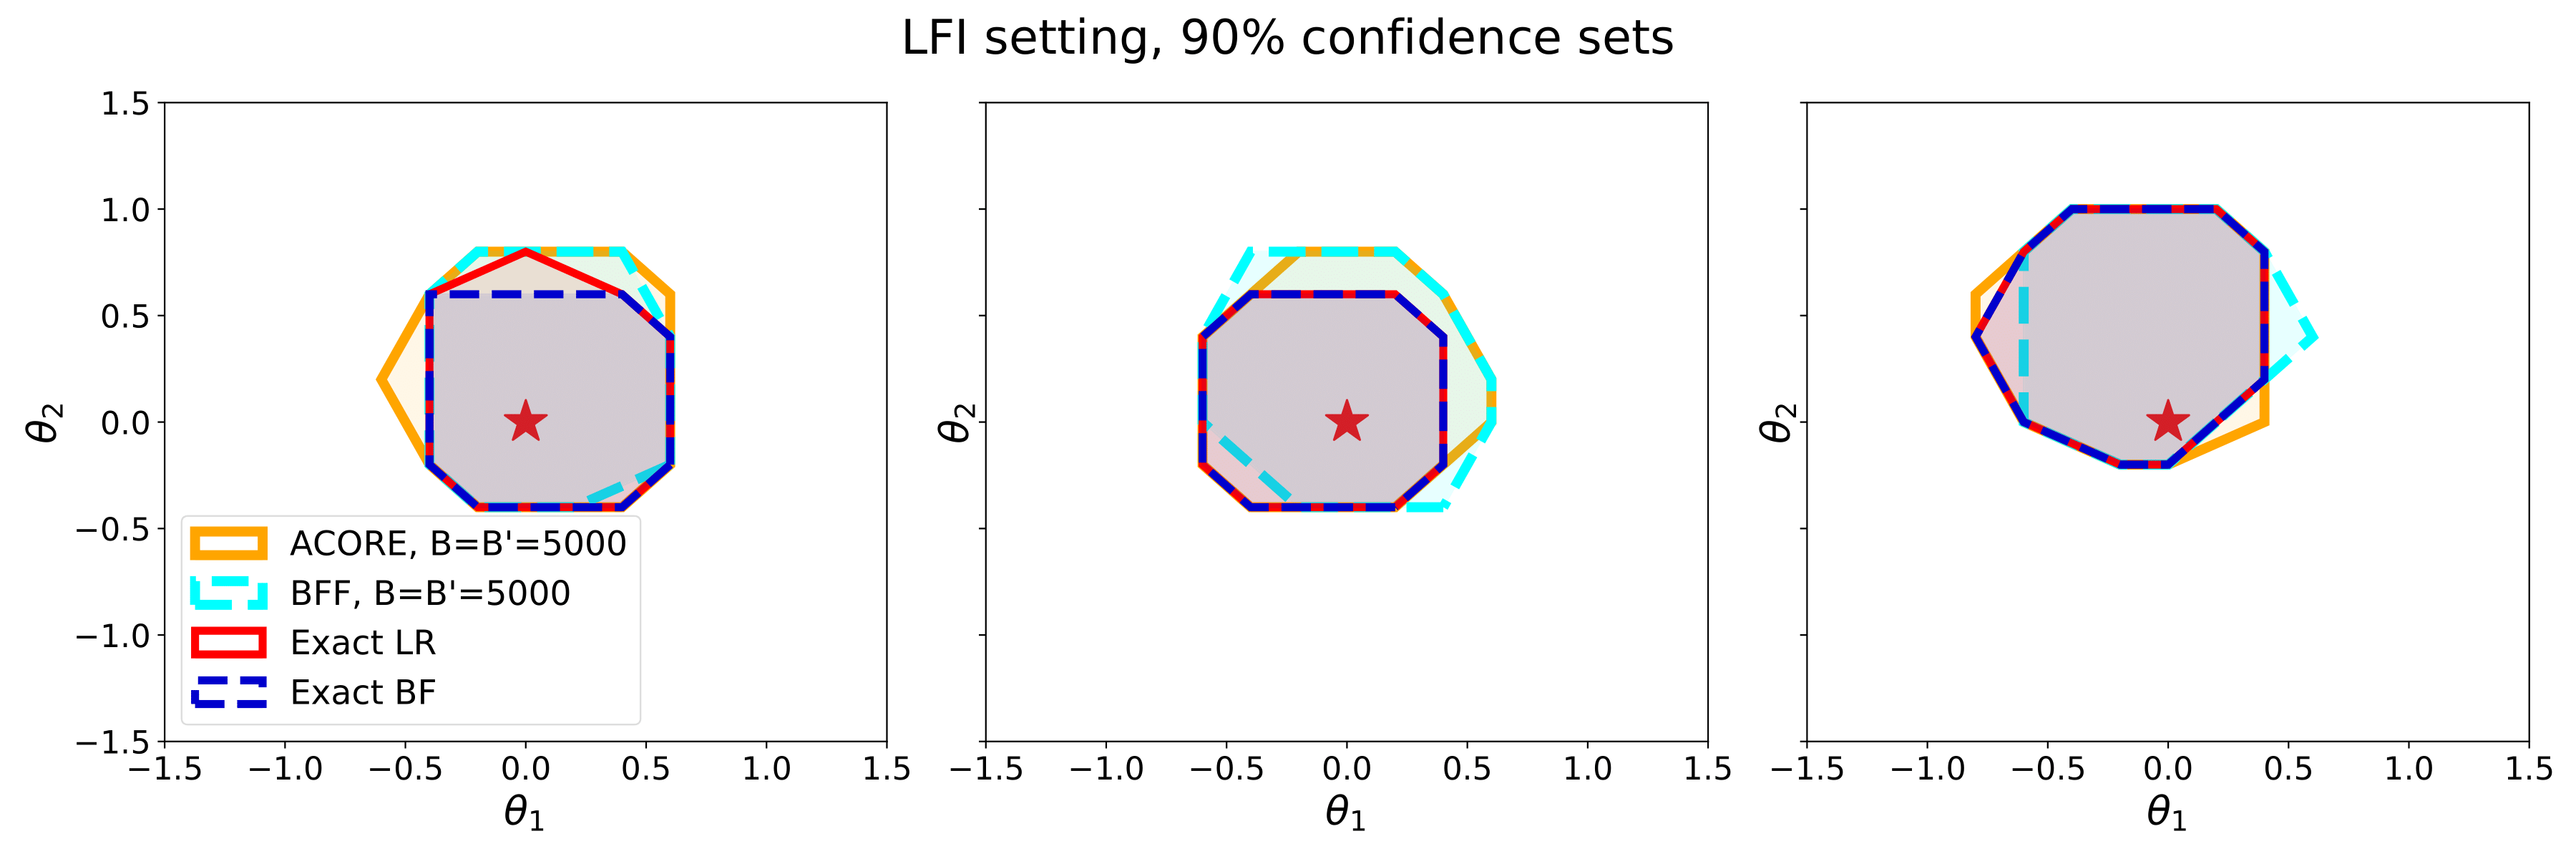}
	\caption{\small  LFI setting: When $d=2$, \texttt{BFF} and \texttt{ACORE} 90\% confidence sets are of similar size to those constructed using the exact LR and BF. The true parameter $\theta = (0,0)$ (indicated with a star),
	$n=10$ observations, $B=B'=5000$ and $M=2500$ samples for \texttt{BFF} and \texttt{ACORE}.
	The figures show three random realizations of the observed data. 
	}
	\label{fig:LFI_CIs}
\end{figure}

\begin{figure}[b!]
	\centering
	\textbf{Finite-sample confidence sets in a likelihood-free inference setting} 
	\par\medskip
    \vspace*{-1mm}
	\begin{tabular}{|c|c|c|c|c|}
		\hline
		& \textbf{d=1} & \textbf{d=2} & \textbf{d=5} & \textbf{d=10} \\ \hline
        \textbf{Coverage of \ACORE} & 0.92 $\pm$ 0.03 & 0.92 $\pm$ 0.03 & 0.90 $\pm$ 0.03 & 0.90 $\pm$ 0.03 \\ \hline
        \textbf{Coverage of \BFF} & 0.94 $\pm$ 0.02 & 0.89 $\pm$ 0.03 & 0.96 $\pm$ 0.02 & 0.87 $\pm$ 0.03\\ \hline
	\end{tabular}
    \includegraphics[width=0.925\textwidth]{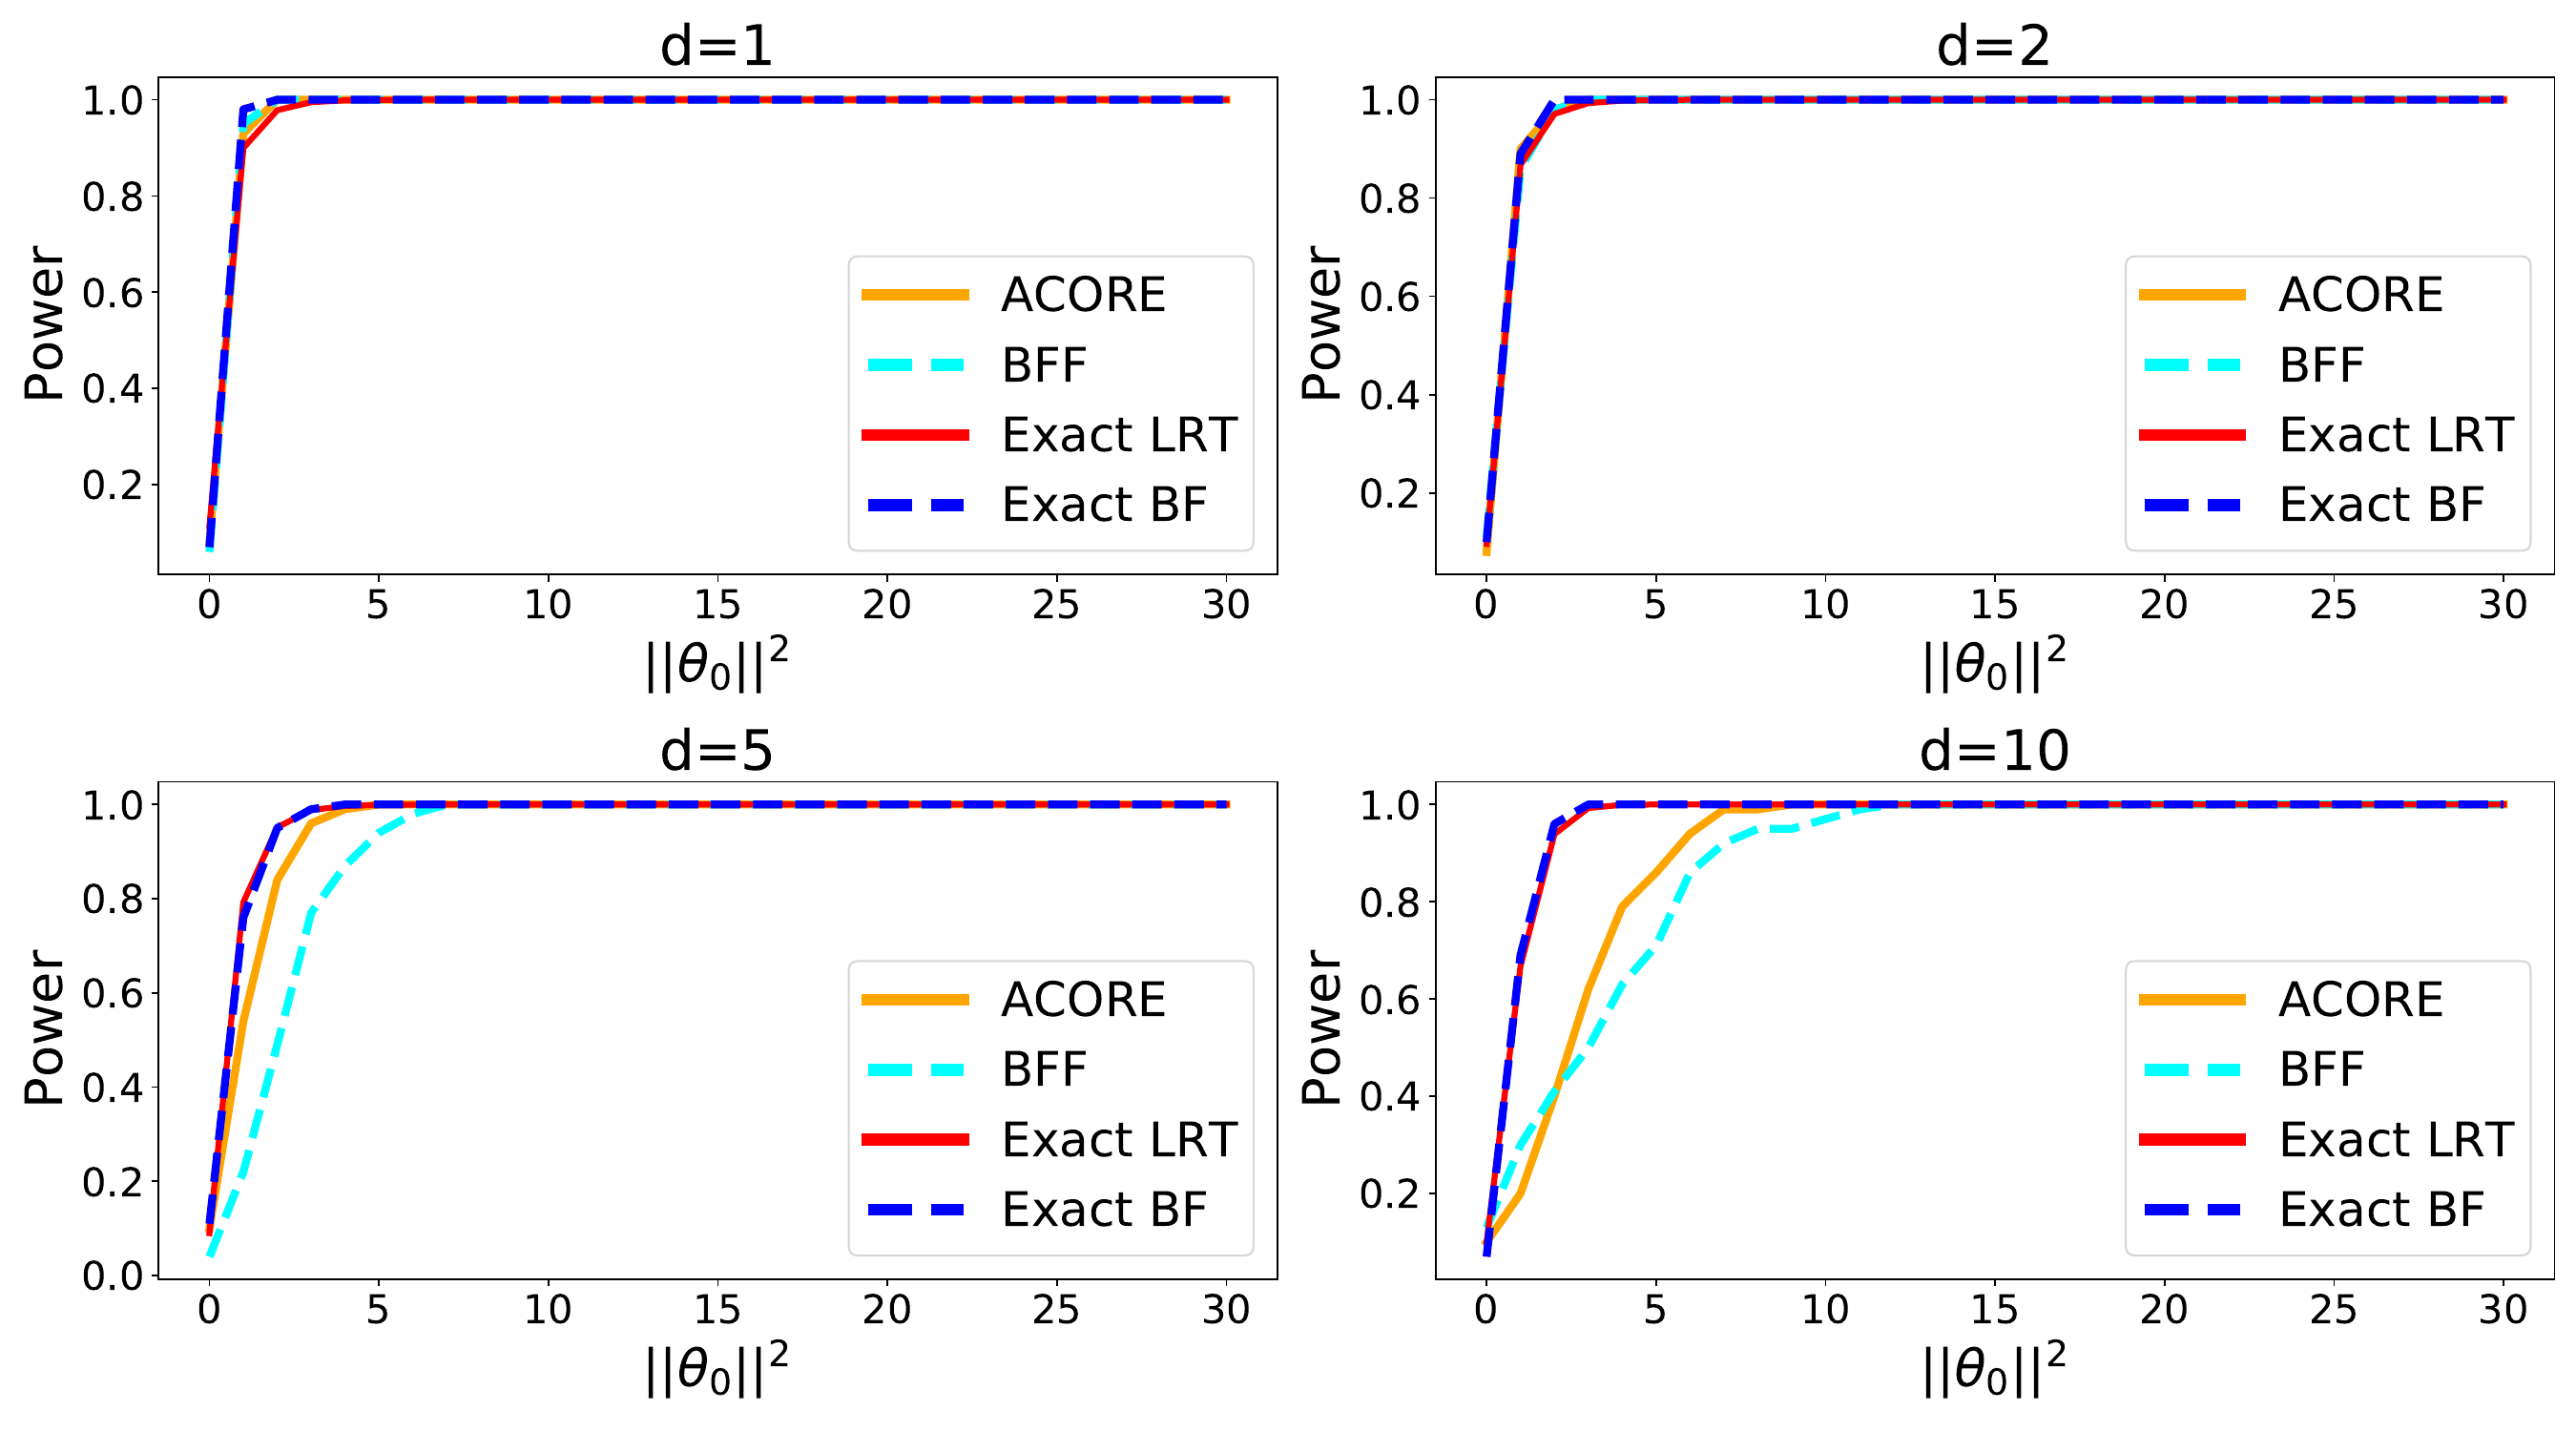} \\
	\caption{
	\small 
	 LFI setting: Coverage and power for \ACORE and \BFF confidence sets and their exact likelihood ratio test (LRT) and Bayes factor (BF) counterparts at dimension $d=1,2,5$ and $10$ across 100 repetitions. Both \ACORE and \BFF return valid confidence sets with coverage at or above the nominal confidence level $1-\alpha=0.9$. The loss in power relative the exact methods increases as $d$ increases.  (We use QDA to learn the odds, with sample size $B$ guided by Figure~\ref{fig:gaussian_isotropic_banalysis}, a computational budget for maximization and integration of $M=10000$, and quantile regression gradient boosting trees with $B^{'}=10000$.)
	}
	\label{fig:gaussian_LFI_power_acrossd}
\end{figure}

In this section, we assess how our procedures scale with parameter and feature dimension for the (analytically solvable) problem of estimating the population mean of $d$-dimensional Gaussian data. 
(This is an example where we can analytically derive test statistics as well as the exact null distribution of the LR statistic.)  In Supplementary Material~\ref{sec:mvn_example_knownlik}, we first assume that the LR statistic is known but not its null distribution, so that we can compare our calibrated confidence sets to universal inference sets and the exact (uniformly most powerful) LR confidence sets. Thereafter, in Supplementary Material~\ref{sec:mvn_example_LFI}, we consider the standard LFI setting with a likelihood that is only implicitly encoded by the simulator.

For the multivariate Gaussian (MVG) example, suppose $\X_1,\ldots,\X_n \sim N(\theta, I_d)$, where $I_d$ is the $d$-dimensional identity matrix and $\theta \in \mathbb{R}^d$ is an unknown parameter.
 For this model, the sample mean $\overline{\X}_n \sim N(\theta,n^{-1}I_d )$ is a sufficient statistic, so we can express our test statistics in terms of $\overline{\X}_n$. 
  The likelihood ratio statistic for testing
  $H_{0, \theta_0}: \theta = \theta_0$ versus $H_{1, \theta_0}: \theta \neq \theta_0$ is
\begin{equation}\label{eq::LRT_MVN}
    \text{LR}(\overline{\X}_n; \theta_0) = 
    \log \frac{N(\overline{\X}_n;\theta_0, n^{-1}I_d)}  {N(\overline{\X}_n;\overline{\X}_n, n^{-1}I_d)} = - \frac{n}{2} \|\overline{\X}_n - \theta_0  \|^2.
\end{equation}
For the MVG example, it holds exactly that  $-2\text{LR}(\overline{\X}_n;\theta_0) \sim \chi^2_d$. We refer to inference based on the above result as ``exact LRT''. For example, the exact LRT confidence set at level $\alpha$ is defined as
$$R^{\text{LRT}}(\overline{\X}_n) = \{ \theta_0 \in \Theta :  n \|\bar{\X}_n - \theta_0  \|^2 \leq c_{\alpha,d}\},$$ where $c_{\alpha, d}$ is the upper $\alpha$ quantile of a $\chi^2_d$ distribution.

For the Bayes factor, we assume a proposal distribution $\pi$ that is uniform over an axis-aligned hyper-rectangle with corner points at $\textbf{a} = (a,...,a)$ and $\textbf{b} = (b,...,b) \in \mathbb{R}^d$ for $a<b$.
The exact Bayes factor for testing 
$H_{0, \theta_0}: \theta = \theta_0$ versus $H_{1, \theta_0}: \theta \neq \theta_0$ is
\begin{align}
    {\rm BF}(\overline{\X}_n; \theta_0) = \frac{N(\overline{\X}_n;\theta_0, n^{-1}I_d)}{\left(\frac{1}{b-a}\right)^d \prod_{j=1}^d \left[ \frac{1}{2} {\rm erf}\left(\frac{b - \overline{X}_{n,j}}{\sqrt{2n}} \right) - \frac{1}{2}{\rm erf}\left(\frac{a - \overline{X}_{n,j}}{\sqrt{2n}} \right) \right]}.
\end{align}
See Supplementary Material~\ref{app:sim_derivs} for a derivation. We refer to inference based on the above expression and high-resolution Monte Carlo sampling  to compute critical values as ``exact BF''.

With the exact LRT and exact BF  as benchmarks, we \revJMLR{can} assess the coverage and power of our LFI constructed confidence sets with increasing parameter and feature dimension $d$.

\subsection{Finite-Sample Confidence Sets for Known Test Statistic}\label{sec:mvn_example_knownlik}
We start with an LFI setting where we assume the test statistic is known, but not its null distribution and critical values.  
Recently, \cite{wasserman2020universal} proposed a general set of procedures for constructing confidence sets and hypothesis tests with finite-sample guarantees. One instance of universal inference uses the crossfit likelihood-ratio test, which averages the likelihood ratio statistic over two data splits; see also recent work by \cite{dunn2021gaussian}, which compares different universal inference schemes on MVG data.  Our LFI approach can also produce valid finite-sample confidence sets for known test statistic by calibrating the critical value as in Algorithm 1. 

Figure~\ref{fig:known_CIs} compares three ``Exact LRT'' sets with confidence sets constructed with our method for estimating the critical value (``LR with calibrated C''), and confidence sets via universal inference with crossfit LRT (``Universal Inference LRT''). 
The dimension here is $d=2$, the true (unknown) parameter is $\theta^*=(0,0)$, and the sample size is $n=10$. By calibrating the critical value, we can achieve valid confidence sets similar to exact LRT for a modest number of  $B'=500$ simulations. Universal inference does not adjust the critical values according to the value of $\theta$, and pays a price for its generality in terms of larger confidence sets and lower power.

Figure~\ref{fig:MVN_knownlik} extends the comparison to coverage and power in higher dimensions $d$. As before, we observe a sample of size $n=10$ from a MVG centered at
 \revJMLR{$\theta^*=\mathbf{0}$}. We construct confidence sets using exact LRT, LR with calibrated C, and universal inference with crossfit LRT for 100 draws from the MVG. We then test  $H_{0,\theta_0}:\theta=\theta_0$ versus $H_{1,\theta_0}: \theta \neq \theta_0$  for different values of $\theta_0$ at increasing distance $\|\theta_0\|$ from the origin. We reject  $H_{0,\theta_0}$  if $\theta_0$ is outside the constructed confidence set. In this example, coverage is measured by the proportion of times the parameter value $\theta_0=\boldsymbol{0}$ is (correctly) included in the confidence set over 100 such repetitions. Similarly, power is measured by the proportion of times a parameter value $\theta_0 \neq \boldsymbol{0}$ is (correctly) outside the constructed confidence set. For better visualization, we have chosen the test points $\theta_0$ so that we have roughly an equal number of test points at each squared distance $\|\theta_0\|^2$.

The table at the top of the figure shows that both ``LR with calibrated C'' and ``Universal Inference LRT'' control the type I error at level $\alpha=0.1$  for dimensions d between 10 to 100. Universal inference, however, tends to be overly conservative. As for the two-dimensional example, our method achieves almost the same power as the exact LR test, even for $d=100$ and a modest budget of $B'=5000$ simulations. Universal inference has much lower power, as expected. The differences in power between the two methods grows with increasing dimension $d$.

\subsection{Finite-Sample Confidence Sets in an LFI Setting}\label{sec:mvn_example_LFI}

Next, we consider the more challenging LFI scenario where one is only able to sample data from a forward simulator $F_\theta$, and hence needs to estimate {\em both} the test statistic and critical values. As before, we simulate observed data of sample size $n=10$ from a $d$-dimensional Gaussian distribution with true mean $\theta^*=\mathbf{0}$, but now we estimate both the test statistics and the critical values for controlling the type I error. We use \ACORE to approximate the LRT, and \BFF to approximate tests based on the Bayes factor with a uniform prior over the hyper-rectangle $[-5,5]^d$.

Following the strategy outlined in Supplementary Material~\ref{sec:sources_errors}, we select a quadratic discriminant analysis (QDA) classifier to estimate the odds, and quantile regression with gradient boosted trees to estimate cutoffs  at level $\alpha=0.1$. Figure~\ref{fig:LFI_CIs} compares \ACORE and \BFF confidence sets when $d=2$ to the exact LRT and exact BF counterparts (achieved with computationally expensive MC sampling to estimate critical values). Both \ACORE and \BFF achieve similarly sized confidence sets as their exact counterparts, with modest budgets of $B=B'=5000$ simulations and $M=2500$ evaluation points for maximization or integration.

Figure~\ref{fig:gaussian_LFI_power_acrossd} shows the coverage and power of these methods as the dimension $d$ increases. We use the same approach as in Supplementary Material~\ref{sec:mvn_example_knownlik} to compute the power over 100 repetitions. First, we observe that both \ACORE and \BFF confidence sets consistently achieve the nominal $0.90$ confidence level,\footnote{The coverage falls within or above expected variation for $100$ repetitions, which is in the range [84, 95].} even in higher dimensions. Next, we consider power. Loosely speaking, the exact LRT and BF power curves can be seen as upper bounds on the power of \ACORE and \texttt{BFF}, respectively. The results indicate that \ACORE and \BFF confidence sets are precise in low dimensions, but their power drops as $d$ increases.

A closer look (see Supplementary Material~\ref{sec:mvg_details}) indicates that the loss in power for $d \geq 5$ is primarily due to numerical error in the maximization or integration step  (referred to as error $e_2$ in Supplementary Material~\ref{sec:sources_errors}) of \ACORE and \texttt{BFF}, respectively. Hence, we foresee that the current implementations of \ACORE and \BFF with uniformly spaced evaluation points would significantly benefit from more efficient numerical computation. For maximization, higher efficiency approaches have been suggested in the hyper-parameter search literature for machine learning algorithms, such as kernel-based Bayesian optimization \citep{Kandasamy2015BayesOpt} and bandit-based approaches \citep{li2018hyperband} (see \cite{Feurer2019} for an overview). For integration, one could employ more efficient approaches that rely on, e.g., adaptive sampling \citep{lepage1978vegas, jadach2003foam}, nested sampling \citep{Feroz2009multinest, Handley2015polychord} or machine learning algorithms \citep{Bendavid2017mcintegration, Gao2020iflow}.

Here we provide (i) the analytical derivations for the marginal distribution and Bayes factor in the multivariate Gaussian setting, and (ii) Supplementary Material~\ref{sec:mvn_example_LFI}  details for the probabilistic classifier selection and the analysis of  the drop in power for \ACORE and \BFF  at $d=5$ and $d=10$.

\subsection{Analytical Derivations}\label{app:sim_derivs}

Given that the covariance matrix is $\Sigma = I_d$ in this setting, the marginal distribution $F_\X$ has a closed form solution for any $\textbf{a}, \textbf{b} \in \mathbb{R}^d$, which can be expressed as follows:

\begin{align*}
    F_\X (\x) &= \int_{\textbf{a}}^{\textbf{b}} (2\pi)^{-\frac{d}{2}} {\rm det}(\Sigma)^{-\frac{1}{2}} \exp\left(-\frac{1}{2} (\x - \boldsymbol{\mu})^T \Sigma^{-1} (\x-\boldsymbol{\mu})\right) d\boldsymbol{\mu}\\
    &= \int_{\textbf{a}}^{\textbf{b}} (2\pi)^{-\frac{d}{2}} \exp\left(-\frac{1}{2} \left(\sum_{i=1}^d x_i^2 - 2x_i\mu_i + \mu_i^2 \right) \right) d\mu_1 d\mu_2 ... d\mu_d \\
    &= \prod_{i=1}^d \left[ \int_{a_i}^{b_i} (2\pi)^{-\frac{1}{2}} \exp\left(-\frac{1}{2} x_i^2 + x_i\mu_i -\frac{1}{2} \mu_i^2 \right) d\mu_i \right] \\
    &= \prod_{i=1}^d \frac{1}{2} {\rm erf}\left(\frac{b_i - x_i}{\sqrt{2}} \right) - \frac{1}{2}{\rm erf}\left(\frac{a_i - x_i}{\sqrt{2}} \right),
\end{align*}

In this setting, the proposal distribution $\pi$ is uniform over an axis-aligned hyper-rectangle with extremes $\textbf{a} = (a, ..., a)$ and $\textbf{b} = (b, ..., b)$ for $a < b \in \mathbb{R}$. Since $\overline{\mathbf{X}}_n$ is a sufficient statistic, the exact Bayes factor for the Neyman construction when testing $H_{0, \theta_0}: \theta = \theta_0$ versus $H_{1, \theta_0}: \theta \neq \theta_0$ is equal to:

\begin{align*}
    \rm{BF}(\mathcal{D}; \theta_0) &= \frac{N(\overline{\X}_n;\theta_0, n^{-1}I_d)}{\int_{\textbf{a}}^{\textbf{b}} N(\overline{\X}_n;\theta, n^{-1}I_d) d\pi(\theta)} \\
    &= \frac{N(\overline{\X}_n;\theta_0, n^{-1}I_d)}{\left(\frac{1}{b-a}\right)^d \int_{\textbf{a}}^{\textbf{b}} N(\overline{\X}_n;\theta, n^{-1}I_d) d\theta} \\
    &= \frac{N(\overline{\X}_n;\theta_0, n^{-1}I_d)}{\left(\frac{1}{b-a}\right)^d \prod_{j=1}^d \left[ \frac{1}{2} {\rm erf}\left(\frac{b - \overline{X}_{n,j}}{\sqrt{2n}} \right) - \frac{1}{2}{\rm erf}\left(\frac{a - \overline{X}_{n,j}}{\sqrt{2n}} \right) \right]},
\end{align*}
where $\overline{X}_{n,j}$ is the j-th coordinate of $\overline{\mathbf{X}}_n$.

\subsection{Details on Section~\ref{sec:mvn_example_LFI}}\label{sec:mvg_details}

Figure~\ref{fig:gaussian_isotropic_banalysis} (left) compares cross-entropy loss curves for the QDA (the best classifier for the Gaussian likelihood model) and MLP classifiers. As we increase $B$, odds estimation becomes more accurate, and we expect to see a decrease in both cross-entropy loss 
and integrated odds loss, as shown in Figure~\ref{fig:gaussian_isotropic_banalysis} (right). 

\begin{figure*}[!ht]
    \centering
    \includegraphics[width=1.03\textwidth]{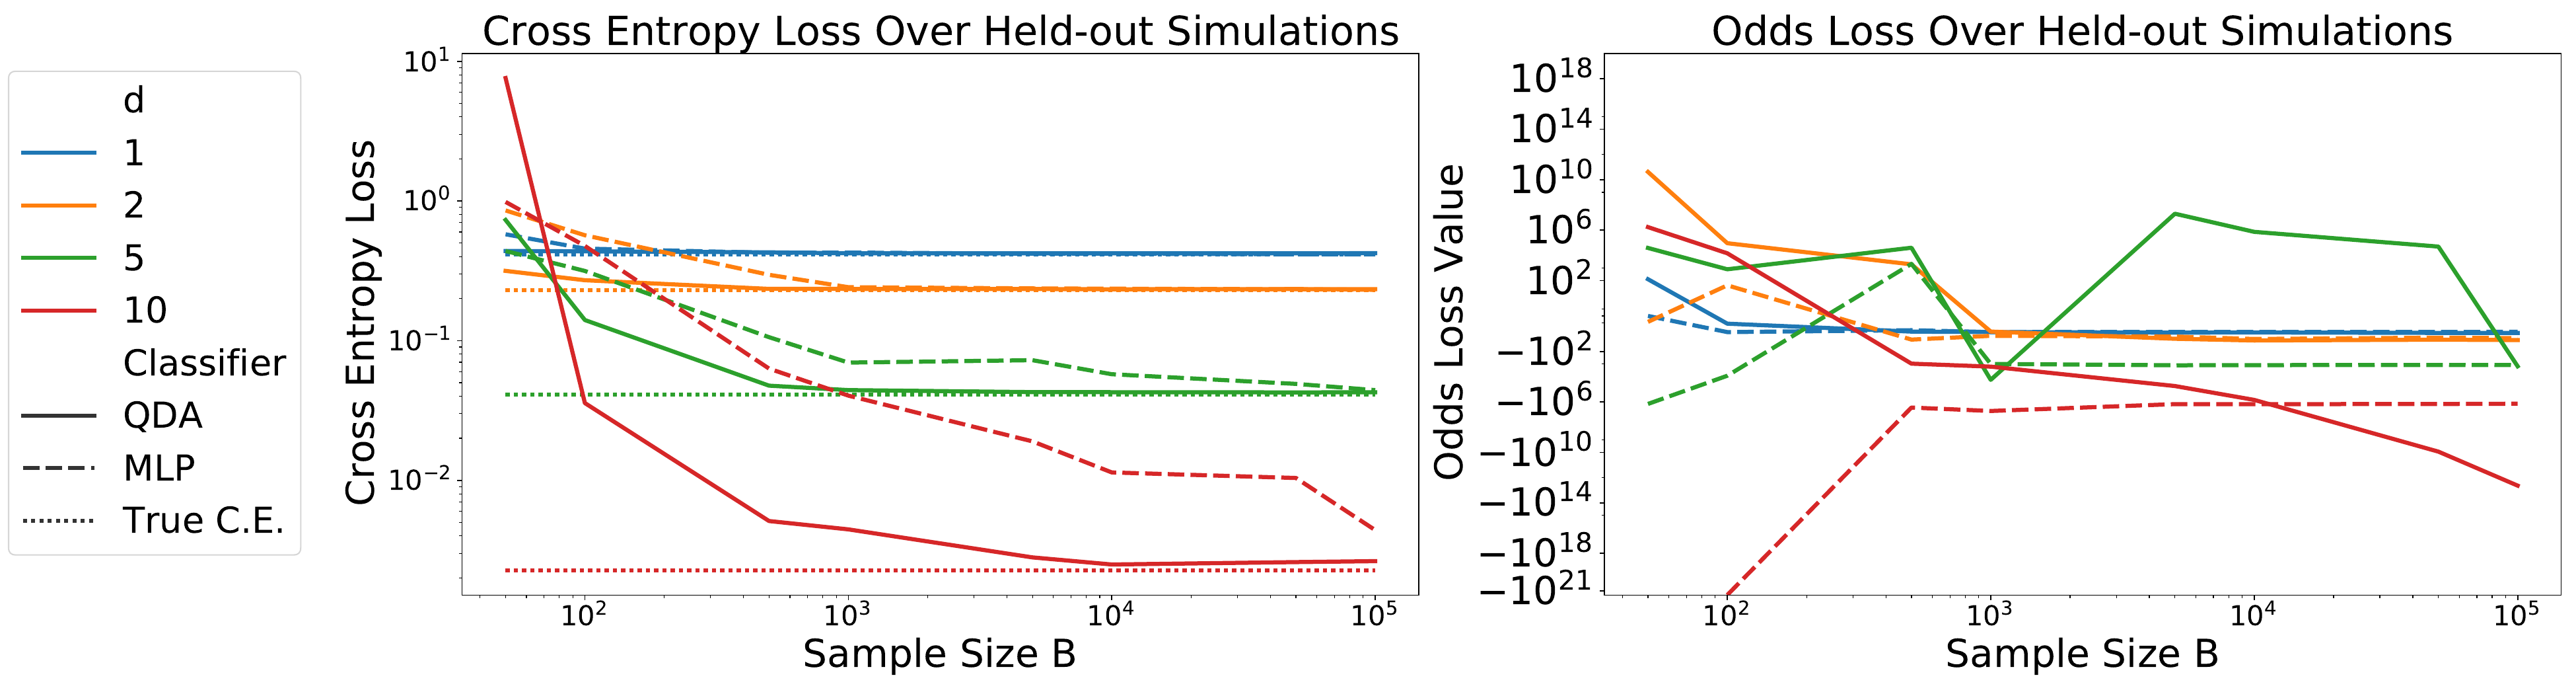}
    \caption{\small \textit{Left}: Cross-entropy loss in learning the odds versus the sample size $B$ (Algorithm~\ref{alg:joint_y}) for a QDA and MLP classifier, as well as the true cross entropy, for the Gaussian likelihood model in dimensions $d=1,2,5$ and $10$. QDA has the lowest cross-entropy loss among the classifiers we considered (of which MLP is one example). The values $B$ at which the cross entropy plateaus are used as the sample sizes for learning the odds at various dimensions. \text{Right}: The integrated odds loss generally decreases with increasing $B$, as expected, though it is noisier (the presence of small probabilities blows up the odds ratio). For larger values of $B$, the integrated odds loss should be more stable.}
    \label{fig:gaussian_isotropic_banalysis}
\end{figure*}

We showed in Section \ref{sec:theory} that the power of \texttt{BFF} is bounded by the integrated odds loss. In practice, this loss may be more stably estimated for larger $B$, which would make it an attractive alternative to the cross-entropy loss. The performance difference in Figure~\ref{fig:gaussian_isotropic_banalysis} is reflected in Figure~\ref{fig:odds_est}, highlighting the importance of choosing the best fitting classifier.

\begin{figure*}[b!]
    \centering
    \includegraphics[width=6.0cm, valign=t]{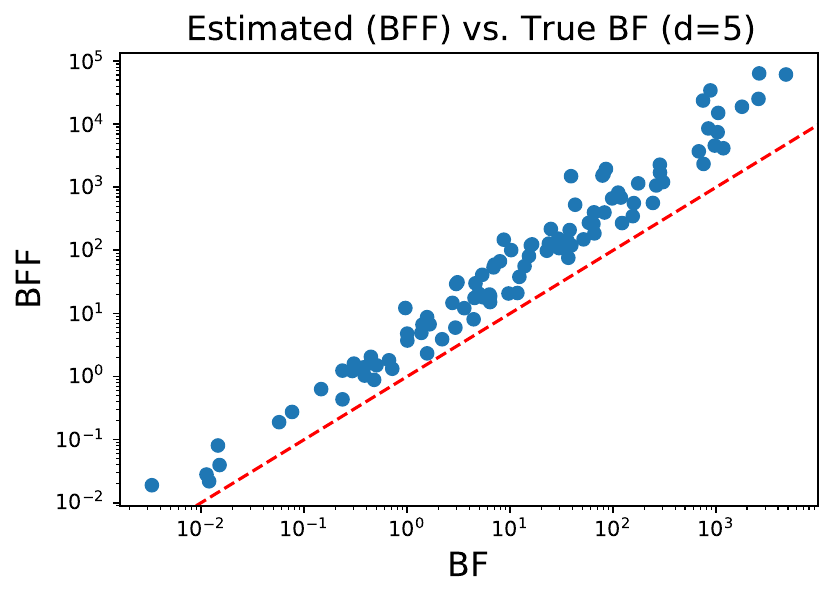}
    \includegraphics[width=6.0cm, valign=t]{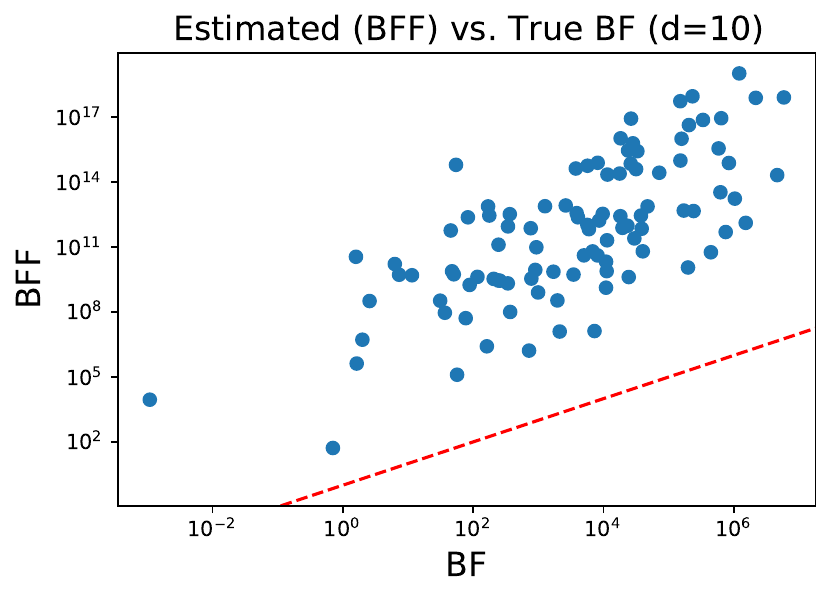}
    \includegraphics[width=6.0cm, valign=t]{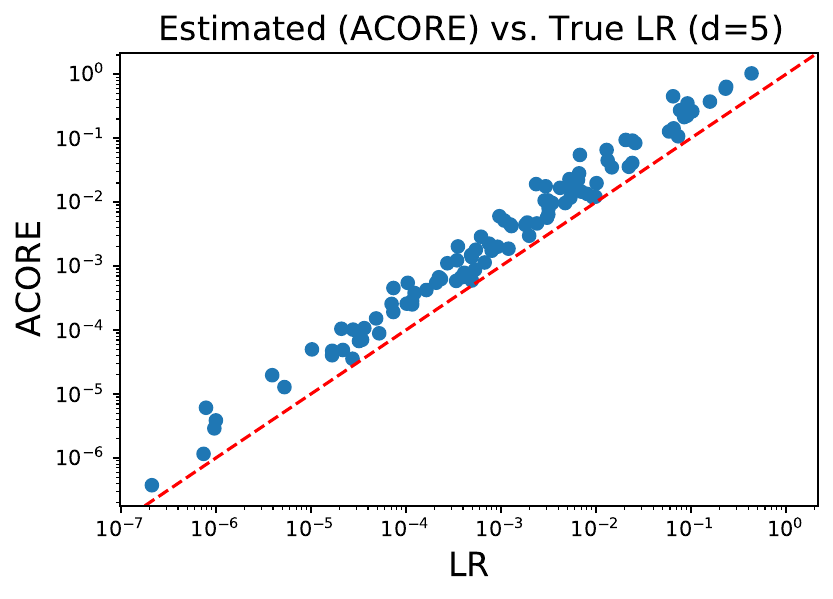}
    \includegraphics[width=6.0cm, valign=t]{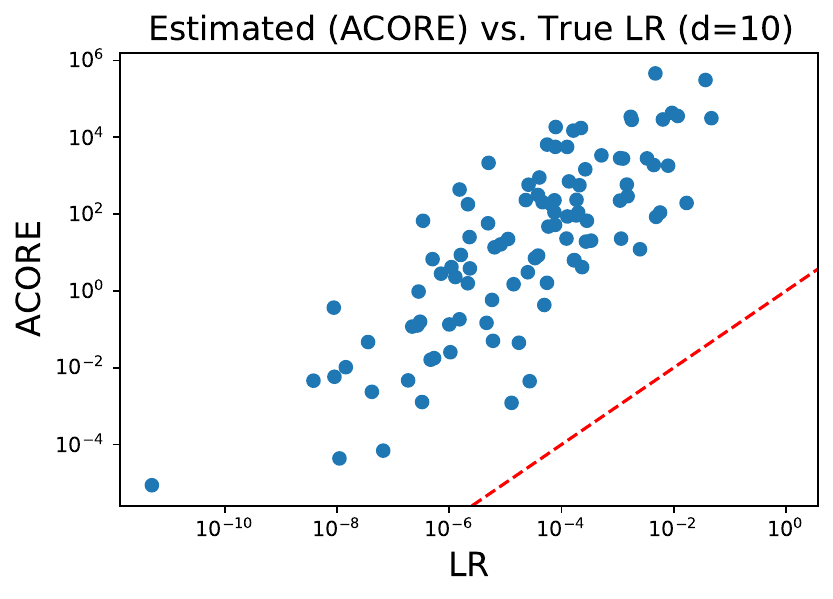}
    \caption{We estimate the \texttt{BFF} and \texttt{ACORE} test statistics using exact odds, so the only error is due to numerical estimation of the denominator with $N=30000$ uniform samples. We see that as $d$ grows, this numerical estimation quickly becomes imprecise, even for large values of $N$.}
    \label{fig:denom_est}
\end{figure*}

\begin{figure*}[t!]
    \centering
    \includegraphics[width=6.2cm, valign=t]{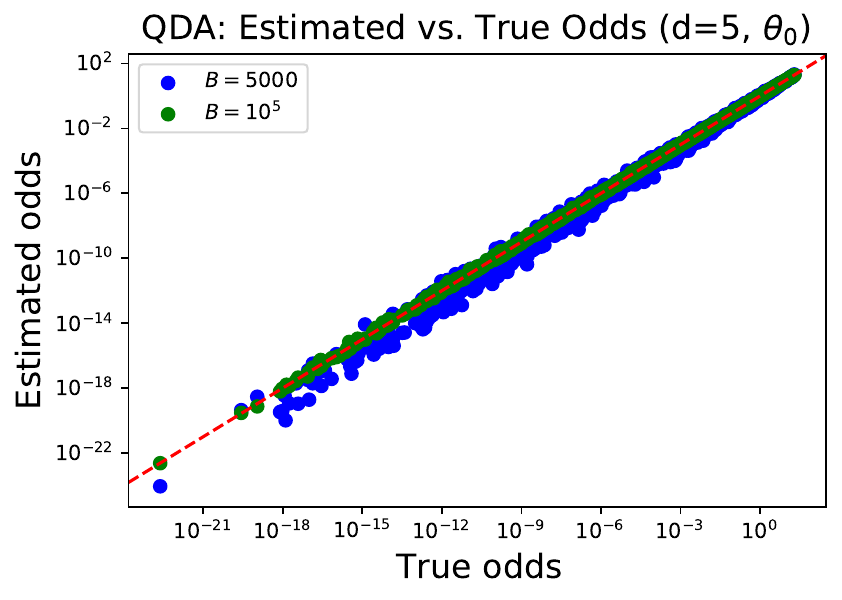}
    \includegraphics[width=6.2cm, valign=t]{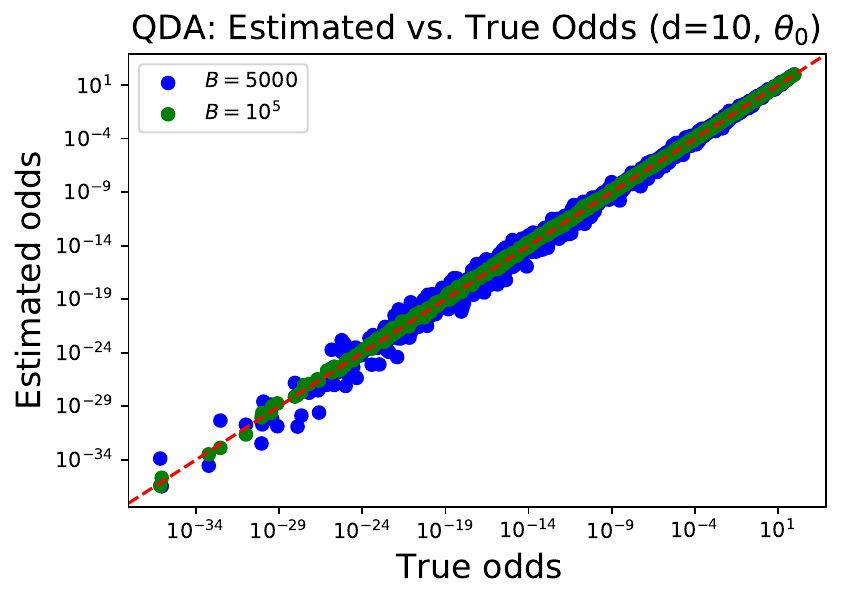}
    \includegraphics[width=6.2cm, valign=t]{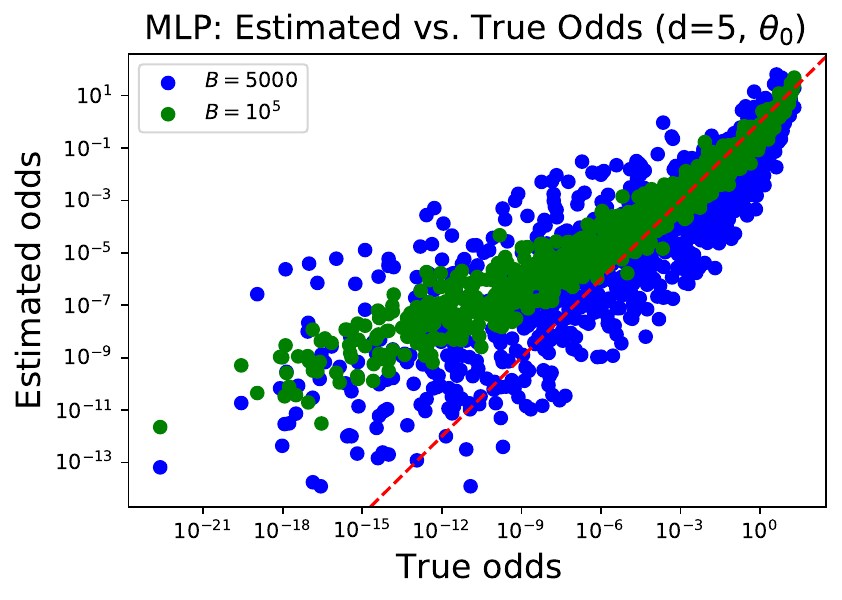}
    \includegraphics[width=6.2cm, valign=t]{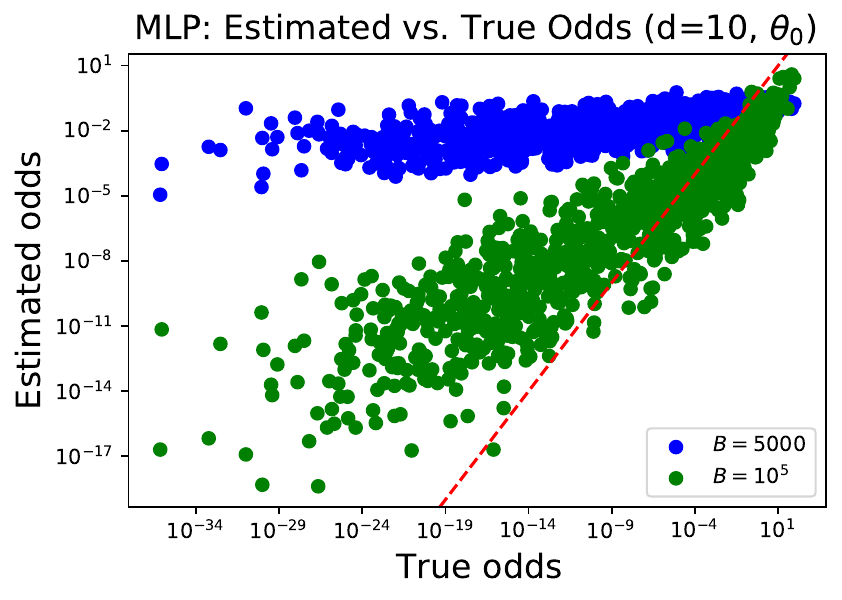}
    \caption{Odds classifiers trained on $B$ samples, evaluated on 1000 test samples. QDA (top row) fits better than MLP (bottom row), and QDA with $B=10^5$ fits well.}
    \label{fig:odds_est}
\end{figure*}

To pinpoint the cause of the degradation in power in high dimensions for \ACORE and \texttt{BFF} in Supplementary Material~\ref{sec:mvn_example_LFI}, we separate the error in estimating the odds from the numerical error in the maximization or integration step for the test statistic (errors $e_1$ and $e_2$ in Supplementary Material~\ref{sec:sources_errors}). Figure~\ref{fig:odds_est} shows that the QDA estimation error is negligible at both $d=5$ and $d=10$ (as opposed to MLP estimation error). To isolate the numerical error, Figure~\ref{fig:denom_est} shows the estimated \ACORE and \BFF statistics using the analytical odds function. Even with a large budget of $M=30000$, we underestimate both the odds maximum and the integrated odds across the parameter space, resulting in an over-estimation of the \ACORE and \BFF test statistics.

\section{Computational Stability for \texttt{BFF}}

When computing the \texttt{BFF} statistics for the Neyman construction hypothesis testing, the denominator is approximated by an average in the following way:

$$
\tau(\D; \theta_0) :=  \frac{  \prod_{i=1}^n  \mathbb{O}(\X_i; \theta_0)}{ \int_{\Theta}  \left(\prod_{i=1}^n  \mathbb{O}(\X_i;\theta) \right) d\pi(\theta)} \approx \frac{  \prod_{i=1}^n  \mathbb{O}(\X_i;\theta_0)}{ \frac{1}{m} \sum_{j=1}^m  \prod_{i=1}^n  \mathbb{O}(\X_i;\theta_j)},
$$
where $\theta_j\sim \pi(\theta)$ for $j=1,...,m$. In practice, the product of odds can quickly run into overflow/underflow. If one assumes $m \leq \mathbb{O}(\X_i;\theta_j) \leq M$ for all $X_i, \theta_j$, the product over $n$ samples can range from $m^n \leq \prod_{i=1}^n \mathbb{O}(\X_i;\theta_j) \leq M^n$ which could be below or above machine precision depending on the values of $m$ and $M$ respectively. Running computations in log-space provides computationally stable calculations even for large samples. First, we can express the test statistic approximation in the following way:

$$
\tau(\D; \theta_0) \approx \frac{  \prod_{i=1}^n  \mathbb{O}(\X_i; \theta_0)}{ \frac{1}{m} \sum_{j=1}^m  \prod_{i=1}^n   \mathbb{O}(\X_i; \theta_j)} = \frac{\exp^{\sum_{i=1}^n \log( \mathbb{O}(\X_i; \theta_0))}}{ \frac{1}{m} \sum_{j=1}^m  \exp^{\sum_{i=1}^n \log( \mathbb{O}(\X_i; \theta_j))}}.
$$

Let $\psi^0 = \sum_{i=1}^n \log(\mathbb{O}(\X_i; \theta_0))$ and $\psi_j = \sum_{i=1}^n \log(\mathbb{O}(\X_i; \theta_j))$. Computing the log-space version of the \texttt{BFF} test statistics then leads to

$$
\log(\tau(\D; \theta_0)) = \psi^0 - \log \left(\frac{1}{m} \sum_{j=1}^m  \exp^{\psi_j} \right) = \psi^0 + \log(m) - \log\left(\sum_{j=1}^m  \exp^{\psi_j} \right).
$$

The above can be made computationally stable by using any of the ``log-sum-exp'' implementations available (such as in \texttt{SciPy}, \cite{2020SciPy-NMeth}).

%\end{supplement}
